# Supplementary material for: Aspects of visible singularities in gravitational collapse
Source: arXiv:2211.06604 source file (2022-11-12)
Supplement: Supplementary file 1 [file AppendixTemplate.tex]

% Appendix Template

\chapter{Local visibility} % Main appendix title

\label{AppendixA} % Change X to a consecutive letter; for referencing this appendix elsewhere, use \ref{AppendixX}

\lhead{Appendix A. \emph{Local visibility}} % Change X to a consecutive letter; this is for the header on each page - perhaps a shortened title

Write your Appendix content here.
